# Supplementary material for: ValuePilot: A Two-Phase Framework for Value-Driven Decision-Making
Source: arXiv:2503.04569 source file (2025-03-06)
Supplement: Supplementary file 1 [file algorithm.tex]

\begin{algorithm}[ht]
\caption{Action Selection Module}
\label{alg:action-selection}
\begin{algorithmic}[1]
\setlength{\jot}{-2pt} % 行间距缩小
\raggedright

\Statex \textbf{Input:}
\Statex $Scenario \ Relevance : \text{P}^s$ = $[\rho^s_1,\ \rho^s_2, \ldots, \rho^s_m]$
\Statex $Actions \ Relevance \ Matrix$ : $[\text{P}^a_1,\ \text{P}^a_2,\ldots,\text{P}^a_n]$
\Statex $Preprocessed \ Value \ Preferences : P' $= $[p'_1,\ p'_2,\ldots,p'_m]$
\Statex \textbf{Parameter:}
\Statex $Scenario$
\Statex $Actions = [action1, action2, action3, \ldots, action\_\textbf{n}]$
\Statex $Values = [value1, value2, value3, \ldots, value\_\textbf{m}]$
\Statex \textbf{Output:} $Ranked \ Actions$
\vspace{-0.5mm}
\Statex
\setlength{\jot}{0pt}  % Reduces space between lines of equations
\Statex \textbf{\# Calculate Overall Ratings (Part 1)}
    \FOR{each action $i \in Actions$}
        \FOR{each value\ $j \in Values$}
            \STATE Calculate \textbf{objective ratings} using:
            \begin{equation} 
            o^s_j = \rho^s_j \quad \text{and} \quad o^{a_i}_j = \rho^{a_i}_j \notag
            \end{equation}
            \STATE Calculate \textbf{subjective bias} using:
            \begin{equation}
                s^s_j = 1 - \left| \left| \rho^s_j \right| - p'_j \right| \quad \text{and} \quad
                s^{a_i}_j = 1 - \left| \left| \rho^{a_i}_j \right| - p'_{j} \right| \notag
            \end{equation}
            \STATE Calculate \textbf{combined ratings} using 
            \begin{align}
                &r^s_j = (s^s_j \times w_s) + (o^s_j \times (1 - w_s)) \notag \quad \text{and} \\ 
                &r_{j}^{a_i} = (s^{a_i}_j \times w_a) + (o^{a_i}_j \times (1 - w_a)) \notag
            \end{align}
        \ENDFOR
    \ENDFOR
\end{algorithmic}
\end{algorithm}

\begin{algorithm}[ht]
\setcounter{algorithm}{1} % 将算法编号设置为1，继续编号
\caption{Action Selection Module (continued)}
\label{alg:action-selection-continued}
\begin{algorithmic}[1]
\setlength{\jot}{-2pt} % 行间距缩小
\raggedright

\Statex \textbf{\# Calculate Overall Ratings (continued)}
    \FOR{each action $i \in Actions$}
        \FOR{each value\ $j \in Values$}
            \STATE Calculate \textbf{individual ratings r} using:
            \begin{equation}
                r_{i,j} = \frac{1}{1 + e^{-\left| r_j^s \right| }} \times r_{j}^{a_i} \notag
            \end{equation}
        \ENDFOR
    \ENDFOR
\vspace{-0.5mm}
\Statex
\Statex \textbf{\# Calculate Flows using PROMETHEE Method}
    \FOR{each action $i \in Actions$}
        \FOR{each action $i' \in Actions$}
            \FOR{$value\ j \in Values$}
                \STATE Calculate \textbf{Preference $V_{ii',j}$} using:
                \begin{equation}
                V_{ii',j} = \frac{1}{1 + e^{-(r_{i,j} - r_{i',j})}} \notag
                \end{equation}
            \ENDFOR
        \ENDFOR
    \ENDFOR
    \FOR{each value $j \in Values$}
        \STATE Calculate \textbf{Weighted Preferences $\Tilde{V_{ii'}}$} using:
        \begin{equation}
        \Tilde{V_{ii'}} = \sum_{j=1}^{m} p'_j \cdot V_{ii',j} \notag
        \end{equation} 
    \ENDFOR
    
    \FOR{each action $i \in Actions$}
        \STATE Calculate $\phi_i$ using: 
        \begin{equation}
            \phi^+_i = \frac{1}{n} \sum_{i' \neq i}^{n} \tilde{V}_{ii'}
            \quad \text{and} \quad 
            \phi^-_i = \frac{1}{n} \sum_{i' \neq i}^{n} \tilde{V}_{i'i}
        \end{equation}
        
        \begin{equation}
        \phi_i = \phi^+_i - \phi^-_i \quad \notag
        \end{equation}
    \ENDFOR
\vspace{-0.5mm}
\Statex
\Statex \textbf{\# Rank Actions}
    \STATE $Ranked Actions$ = Sort($Actions$, key=$\phi_i$)

\end{algorithmic}
\end{algorithm}
