# Supplementary material for: ValuePilot: A Two-Phase Framework for Value-Driven Decision-Making
Source: arXiv:2503.04569 source file (2025-03-06)
Supplement: Supplementary file 2 [file 8_appendix.tex]

\begin{algorithm}[ht]
\caption{Action Selection Module}
\label{alg:action-selection}
\begin{algorithmic}[1]
\raggedright

\Statex \textbf{Input:}
\Statex $Scenario\ Model\ Output : \text{P}^s$ = $[\rho^s_1,\ \rho^s_2, \ldots, \rho^s_m]$
\Statex $Actions\ Model\ Output Matrix$ : $[\text{P}^a_1,\ \text{P}^a_2,\ldots,\text{P}^a_n]$
\Statex $Preprocessed \ Agent's \ Preferences : P' $= $[p'_1,\ p'_2,\ldots,p'_m]$
\Statex \textbf{Parameter:}
\Statex $Scenario$
\Statex $Actions = [action1, action2, action3, \ldots, action\_\textbf{n}]$
\Statex $Values = [value1, value2, value3, \ldots, value\_\textbf{m}]$
\Statex \textbf{Output:} $Ranked \ Actions$

\Statex
\Statex \textbf{\# Calculate Overall Ratings}
    \FOR{each action $i \in Actions$}
        \FOR{each value\ $j \in Values$}
            \STATE Calculate \textbf{objective ratings} using Eq.\eqref{eq:1}\eqref{eq:2}
            \STATE Calculate \textbf{subjective bias} using Eq.\eqref{eq:3}\eqref{eq:4}
            \STATE Calculate \textbf{combined ratings} using Eq.\eqref{eq:5}\eqref{eq:6}
            \STATE Calculate \textbf{individual ratings r} using Eq.\eqref{eq:7}

        \ENDFOR
    \ENDFOR

\Statex
\Statex \textbf{\# Calculate Flows using PROMETHEE Method}
    \FOR{each action $i \in Actions$}
        \FOR{each action $i' \in Actions$}
            \FOR{$value\ j \in Values$}
                \STATE Calculate \textbf{Preference $V_{ii',j}$} using Eq.\eqref{eq:8}
            \ENDFOR
        \ENDFOR
    \ENDFOR
    \FOR{each value $j \in Values$}
        \STATE Calculate \textbf{Weighted Preferences $\Tilde{V_{ii'}}$} using Eq.\eqref{eq:9}
    \ENDFOR
    
    \FOR{each action $i \in Actions$}
        \STATE Calculate $\phi_i$ using Eq.\eqref{eq:10}\eqref{eq:11}\eqref{eq:12}
    \ENDFOR

\Statex
\Statex \textbf{\# Rank Actions}
    \STATE $Ranked Actions$ = Sort($Actions$, key=$\phi_i$)

    \end{algorithmic}
\end{algorithm}

\begin{algorithm}
\caption{Model Training Procedure}
\label{alg:training}
\begin{algorithmic}[1]
\STATE \textbf{Define training order:} [6, 1, 5, 2, 4, 3]
\STATE \textbf{Initialize} number of chunks to \( l \)

\FOR{each chunk $i$ from 0 to \( l \) - 1}
    \STATE Initialize Datasets
    
    \FOR{each \texttt{n} in training order}
        \STATE \texttt{Combine\_Dataset}.\texttt{concat}(\texttt{Dataset}[\texttt{n}]])
        \STATE Initialize early stopping parameters
        
        \FOR{each epoch}
            \STATE Train model, validate model, log metrics, and check for early stopping
            \IF{early stopping criteria are met}
                \STATE Save model
            \ENDIF
        \ENDFOR
    \ENDFOR
\ENDFOR

\end{algorithmic}
\end{algorithm}

Algorithm~\ref{alg:order_sensitive} computes the order-sensitive similarity between two sequences by incrementally comparing their prefixes. At each depth, the similarity is calculated as the ratio of the intersection size to the depth. The final score is the average similarity across all depths. This algorithm highlights the importance of early-order elements in the sequence comparison.

\begin{algorithm}[H]
\caption{Order-Sensitive Similarity Measure}
\label{alg:order_sensitive}
\textbf{Input}: Two sequences \( A \) and \( B \), each of length \( n \) \\
\textbf{Output}: Average similarity score \( S \)
\begin{algorithmic}[1]
\STATE \textbf{Initialize} total\_similarity = 0
\FOR{depth \( d = 1 \) to \( n \)}
    \STATE sublist\_A = first \( d \) elements of \( A \)
    \STATE sublist\_B = first \( d \) elements of \( B \)
    \STATE intersection\_size = size of \( \text{Set(sublist\_A)} \cap \text{Set(sublist\_B)} \)
    \STATE similarity\_at\_depth = intersection\_size / \( d \)
    \STATE total\_similarity += similarity\_at\_depth
\ENDFOR
\STATE \textbf{Compute} \( S = \text{total\_similarity} / n \)
\STATE \textbf{Return} \( S \)
\end{algorithmic}
\end{algorithm}
